# Supplementary material for: Edge-preserving noise for diffusion models
Source: arXiv:2410.01540 source file (2026-04-16)
Supplement: Supplementary file 3 [file appendix_flow_matching_comp.tex]

%!TEX root = ../EGauthorGuidelines-conf-sub.tex

\newcommand{\PlotSingleImage}[1]{%
    % \begin{tikzpicture}[scale=1.165]
        \begin{scope}
            \clip (0,0) -- (2.5,0) -- (2.5,2.5) -- (0,2.5) -- cycle;
            \path[fill overzoom image=figures/#1] (0,0) rectangle (2.5cm,2.5cm);
        \end{scope}
        \draw (0,0) -- (2.5,0) -- (2.5,2.5) -- (0,2.5) -- cycle;
        
    % \end{tikzpicture}%
}


\newcommand{\PlotSingleImageNonSquared}[1]{%
    % \begin{tikzpicture}[scale=1.2]
        \begin{scope}
            \clip (0,0) -- (4,0) -- (4,10) -- (0,10) -- cycle;
            \path[fill overzoom image=figures/#1] (0,0) rectangle (4cm,10cm);
        \end{scope}
        \draw (0,0) -- (4,0) -- (4,10) -- (0,10) -- cycle;
        
    % \end{tikzpicture}%
}



% \newcommand{\PlotSingleImageWithLine}[1]{%
%     % \begin{tikzpicture}[scale=1.165]
%         \begin{scope}
%             \clip (0,0) -- (2.5,0) -- (2.5,2.5) -- (0,2.5) -- cycle;
%             \path[fill overzoom image=figures/#1] (0,0) rectangle (2.5cm,2.5cm);
%         \end{scope}
%         \draw (0,0) -- (2.5,0) -- (2.5,2.5) -- (0,2.5) -- cycle;
%         \draw[dashed] (0, -0.13) -- (2.5, -0.13);
%     % \end{tikzpicture}%
% }


% \newcommand{\TwoColumnFigure}[2]{%
%     \begin{tabular}{c@{\;}c@{}}
%         \hspace*{-2.5mm}
%         \begin{tikzpicture}[scale=0.563]
%             \PlotSingleImage{#1}
%         \end{tikzpicture}
%          & 
%          \begin{tikzpicture}[scale=0.563]
%             \PlotSingleImage{#2}
%         \end{tikzpicture}
%     \end{tabular}%
% }


% define the scale value and use it for all
\newcommand\scalevalue{2.4}    % 0.65, 1.85

%
% \small
\hspace*{-4.0mm}
\begin{tabular}{c@{\;}c@{\;}}

%%%%%%%%%%%%%%%%%%%%%%%%%%%%%%%%%%%%%%%%%
%%%%%%%%%%%%%%%%%%%%%%%%%%%%%%%%%%%%%%%%%
%%%%%%%%%%%%%%%%%%%%%%%%%%%%%%%%%%%%%%%%%
%%%%%%%%%%%%%%%%%%%%%%%%%%%%%%%%%%%%%%%%%
% \vline width 0.7 pt
\begin{tabular}{c@{\;}c@{}}
\begin{tikzpicture}[scale=\scalevalue]
\PlotSingleImage{flow_matching_comparison/vanilla.png}
\end{tikzpicture}
\\[-0.4mm]
Flow matching
\\[-0.4mm]
\end{tabular}
&
%%%%%%%%%%%%%%%%%%%%%%%%%%%%%%%%%%%%%%%%%
%%%%%%%%%%%%%%%%%%%%%%%%%%%%%%%%%%%%%%%%%
%%%%%%%%%%%%%%%%%%%%%%%%%%%%%%%%%%%%%%%%%
%%%%%%%%%%%%%%%%%%%%%%%%%%%%%%%%%%%%%%%%%
% \vline width 0.7 pt
\begin{tabular}{c@{\;}c@{}}
\begin{tikzpicture}[scale=\scalevalue]
\PlotSingleImage{flow_matching_comparison/ep.png}
\end{tikzpicture}
\\[-0.4mm]
Edge-preserving flow matching (ours)
\\[-0.4mm]
\end{tabular}
\end{tabular}
